# Supplementary material for: Instance-based Label Smoothing For Better Calibrated Classification Networks
Source: arXiv:2110.05355 source file (2021-10-11)
Supplement: Supplementary file 1 [file appendix.tex]

\documentclass[conference]{IEEEtran}
\IEEEoverridecommandlockouts
% The preceding line is only needed to identify funding in the first footnote. If that is unneeded, please comment it out.
\usepackage{cite}
\usepackage{amsmath,amssymb,amsfonts}
\usepackage{algorithmic}
\usepackage{microtype}
\usepackage{graphicx}
\usepackage{textcomp}
\usepackage{xcolor}
\usepackage{subfigure}
\usepackage{booktabs} % for professional tables
\usepackage{hyperref}
\usepackage{url}
\usepackage{wrapfig}
\usepackage{graphicx}
\usepackage{multirow}
\usepackage{colortbl}
\usepackage{hhline}
\usepackage{tablefootnote}
\usepackage{resizegather}
\usepackage{cite}
\usepackage{tikz}
\usepackage{mathtools}
\usepackage{amssymb}

%% Self-defined macros
 % just an example

%\newcommand{\TO}[1]{}

\def\BibTeX{{\rm B\kern-.05em{\sc i\kern-.025em b}\kern-.08em
    T\kern-.1667em\lower.7ex\hbox{E}\kern-.125emX}}

\begin{document}

\end{document}
